# Supplementary material for: Investigating the effects Diversity Mechanisms have on Evolutionary Algorithms in Dynamic Environments
Source: arXiv:1610.02732 source file (2016-10-09)
Supplement: Supplementary file 1 [file appendixA.tex]

\chapter{Sources}

[1] Whitley, D. (n.d.). An overview of evolutionary algorithms: Practical issues and common pitfalls. Information and Software Technology, 817-831.

[2] Eiben, A., and Smith, J. (2003). Introduction to evolutionary computing. New York: Springer. 

[3] Friedrich, T., Oliveto, P., Sudholt, D., and Witt, C. (n.d.). Analysis of Diversity-Preserving Mechanisms for Global Exploration. Evolutionary Computation, 455-455. 

[4] Mahfoud, S., and Goldberg, D. (1995). In Niching methods for genetic algorithms (p. 20). Urbana, IL.: University of Illinois.

[5] Mumford, C. (2009). Computational intelligence collaboration, fusion and emergence (p. 54). Berlin: Springer.

[6] Zitzler, E. and Thiele, L. (1998). An Evolutionary Algorithm for Multiob jective Optimization: The Strength Pareto Approach (p. 5-6).
